# Supplementary material for: Emotionalism within People-Oriented Software Design
Source: arXiv:1810.12547 source file (2018-10-30)
Supplement: Supplementary file 1 [file AppendixA.tex]

\appendix
\section{Appendix}
\setcounter{table}{0}

\setcounter{figure}{0} 

%\appendix
%\chapter*{Appendix}
%\renewcommand{\thechapter}{A} 
%\section*{Appendices}

\label{appA}

\begin{figure}[ht]
\small
\centering
\includegraphics [scale=0.48]{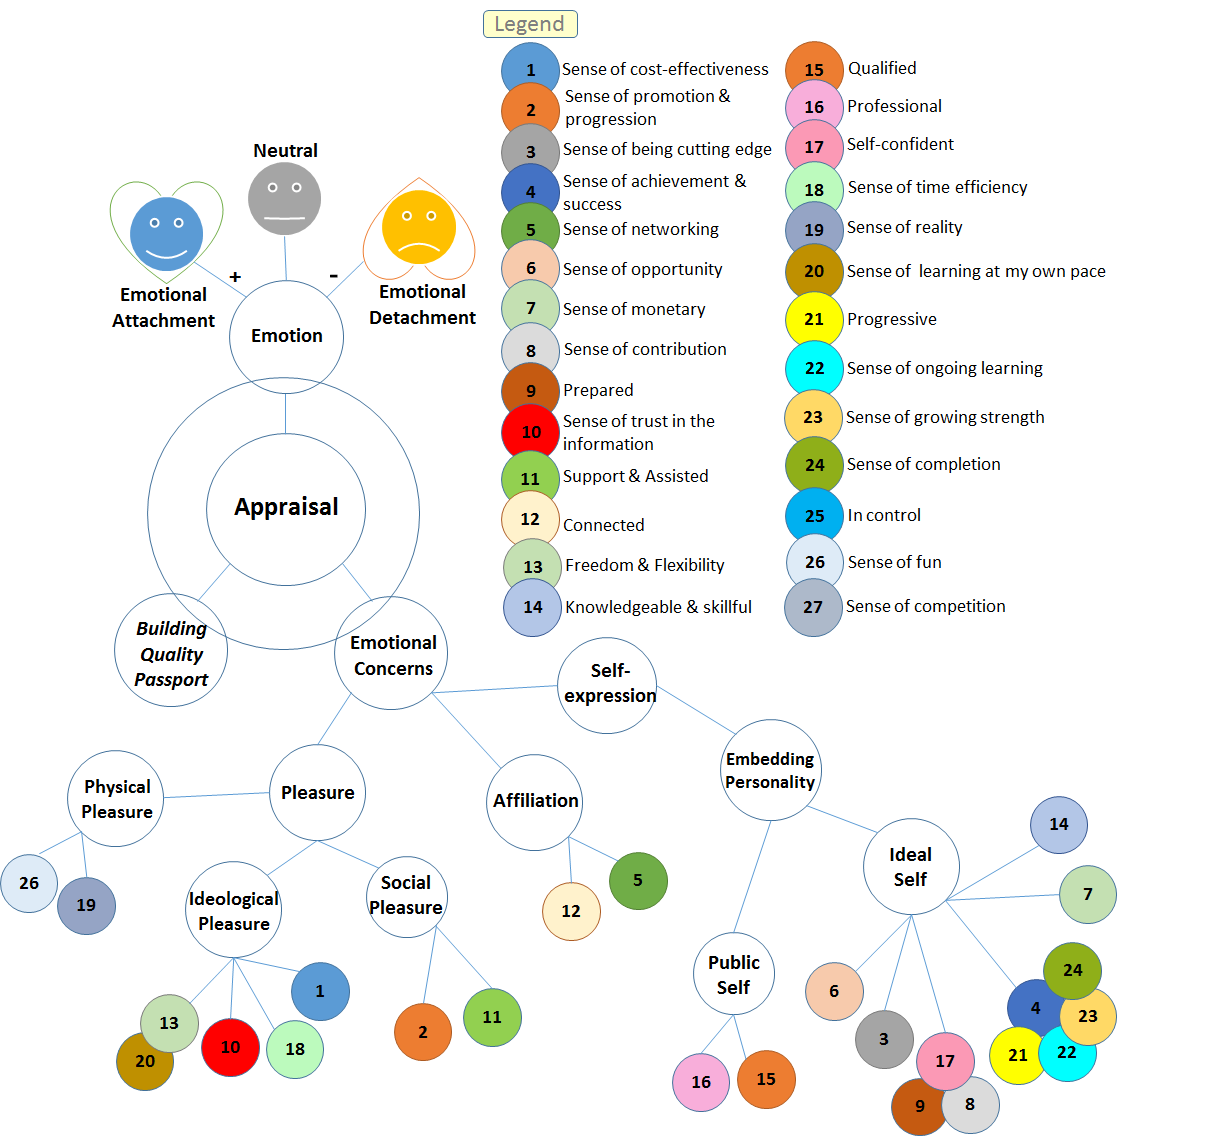}
\caption{\emph{Building Quality Passport} Emotional Goals and Attachment Drivers} 
\label{fig:EAFVQP}
\end{figure}

\begin{landscape}

\begin{table}[]
\centering
\caption{Summary of EQ-FAST Analysis in \emph{Building Quality Passport} Case Study}
\label{emotionalconcerns}

%\resizebox{\textwidth}{!}{%
%\footnotesize
\scriptsize
\begin{tabular}{@{}llll@{}}
\toprule
\textbf{Emotional (Sub-emotional) Goal}  & \textbf{Proposed Quality Goals} & \textbf{Proposed Functional Goals} & \textbf{Comment} \\
\toprule
Freedom and Flexibility & Repeatability, Modularity, Flexible & $-$ & $-$ \\
(Sense of learning at my own pace) \\ (In control) \\
\hline
Sense of time efficiency  & Short and Sharp, Easy to understand, \\  & Reusable Contents, Compatibility / Integrity   &  $-$ & $-$ \\
\hline
Sense of trust in information & Accurate Content, Reliable Platform & $-$ & $-$ \\
\hline
Sense of reality & $-$ & Simulation, Case-based learning & $-$\\
\hline
Knowledgeable \& Skillful & Tangible  & $-$ & Refer to " Sense of reality" \\
\hline
Professional & $-$ & Represent Experiences and Skills, Represent & Refer to "Sense of networking"  \\ &  & Certificates and Qualifications, Like and Follow, & \& "Connected"   \\ && Represent Badges \& Rewards, Represent  \\ && Progress, Networking  \\
\hline
Qualified & $-$ & Represent Experiences and Skills, Represent & Refer to "Sense of networking"  \\ && Certificates \& Qualifications, Like \& Follow,  & \& "Connected" \\ &&  Represent Badges \& Rewards, Represent \\ && Progress, Networking  & \\ 
\hline
Connected & $-$ & Networking & $-$\\
\hline
Supported and assisted  & Easy to find, Instant & Resource, Instructor Feedback & Refer to "Sense of Networking" \\ &&& \& "Connected"\\
\hline
Self-confident & & like and follow & Refer to "Sense of Achievement  \\

(Sense of contribution)&&& and Success",  "Connected",    \\
(Prepared)&&& "Sense of Networking",  \\&&& "Supported and Assisted" \\&&& "Professional" and " Qualified"  \\

\hline
Sense of opportunity  & $-$ & Estimator (Current position, market  \\&& demand, wealth generation) & $-$
 \\
\hline
Sense of monetary (wealth)  & $-$ & $-$ & Refer to "Sense of Networking"  \\ &&&  \& "Connected", \\ &&& "Professional" \& "Qualified" \\
\hline
Sense of achievement \& success & & Benchmarking, Assessment/ Grading,  & Refer to "Professional" \&  \\ (Sense of ongoing learning)&& Goal Planning, Makes progress visible 
(Progressive) & "Qualified" \\
(Sense of completion) && Credentialing Acknowledgement,  \\   &  & Offer Badges \& Reward  \\

\hline
Sense of networking & $-$ & Networking \& Peer Feedback & $-$ \\
\hline
Sense of cost-effectiveness  & Reusable Contents  &  $-$ &  $-$ \\
 \hline
Sense of promotion \& progression   & $-$ & Make progress visible, Benchmarking, Assessment/ & Refer to "Professional" \& \\ &&Grading, Credentialing Acknowledgement, & "Qualified" \\ && Offer Badges and Reward \\
\hline
Sense of being cutting edge & $-$ & Track \& Trace Technology News, Technology & Refer to "Professional" \&  \\ && Statistics and history of use & "Qualified"

 \\
\hline
%In control & $-$ & Flexible  &    $-$  &    $-$  \\
%\hline
Sense of fun & $-$ & Gamification  &  $-$\\
\hline
Sense of competition  &  $-$ & Make progress visible, Benchmarking, Assessment/ & Refer to "Sense of Fun" \\ &&Grading, Credentialing Acknowledgement, \\ && Offer Badges and Reward &    \\

\bottomrule
\end{tabular}% 
%}
\end{table}
\end{landscape}

\begin{landscape}
\begin{figure*}[] 
\small
\centering
\includegraphics [scale=0.48]{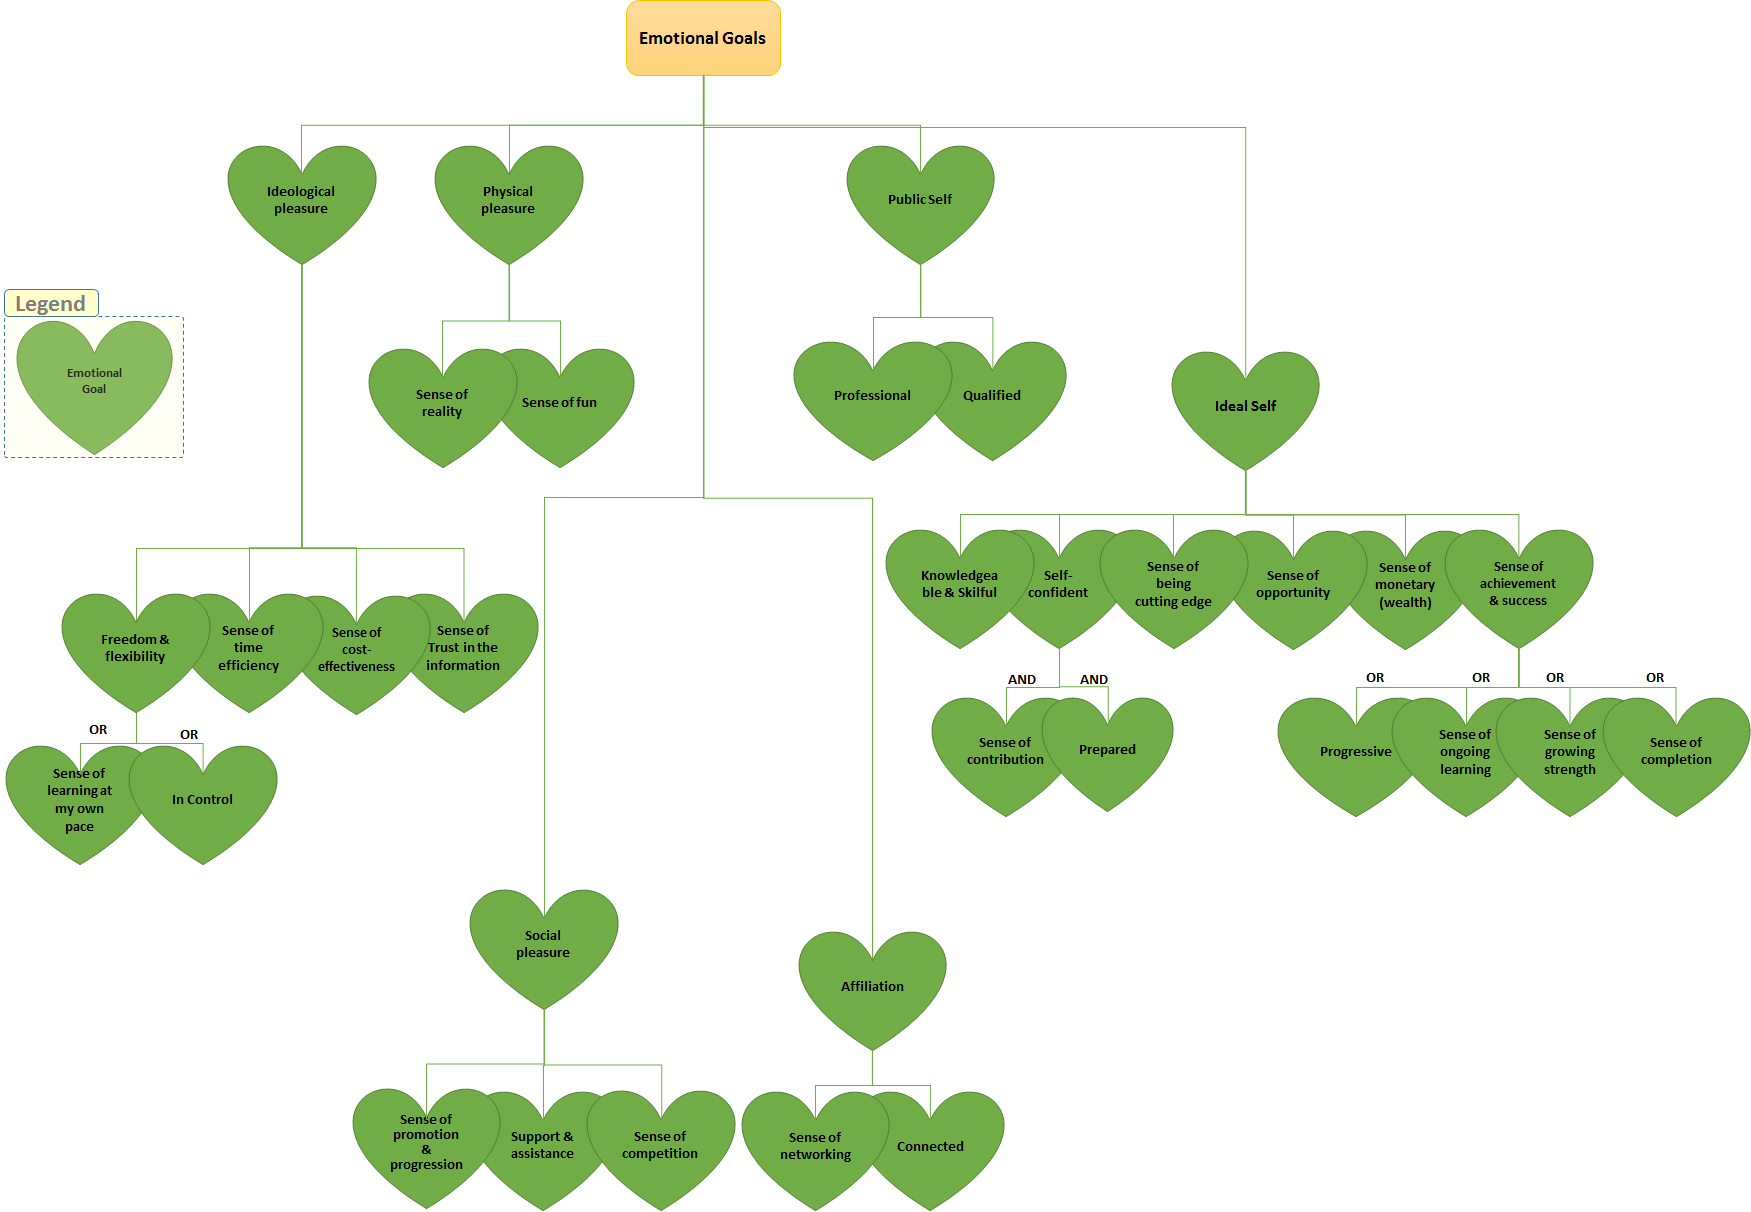}
\caption{\emph{Building Quality Passport} Emotional Goals and Attachment Drivers \\ (\emph{A high-resolution image is available at https://tinyurl.com/y7wtdgbn})}
\label{fig:EGM}
\end{figure*}
\end{landscape}

\begin{landscape}
\begin{figure*}[]
\small
\centering
\includegraphics [scale=0.29]{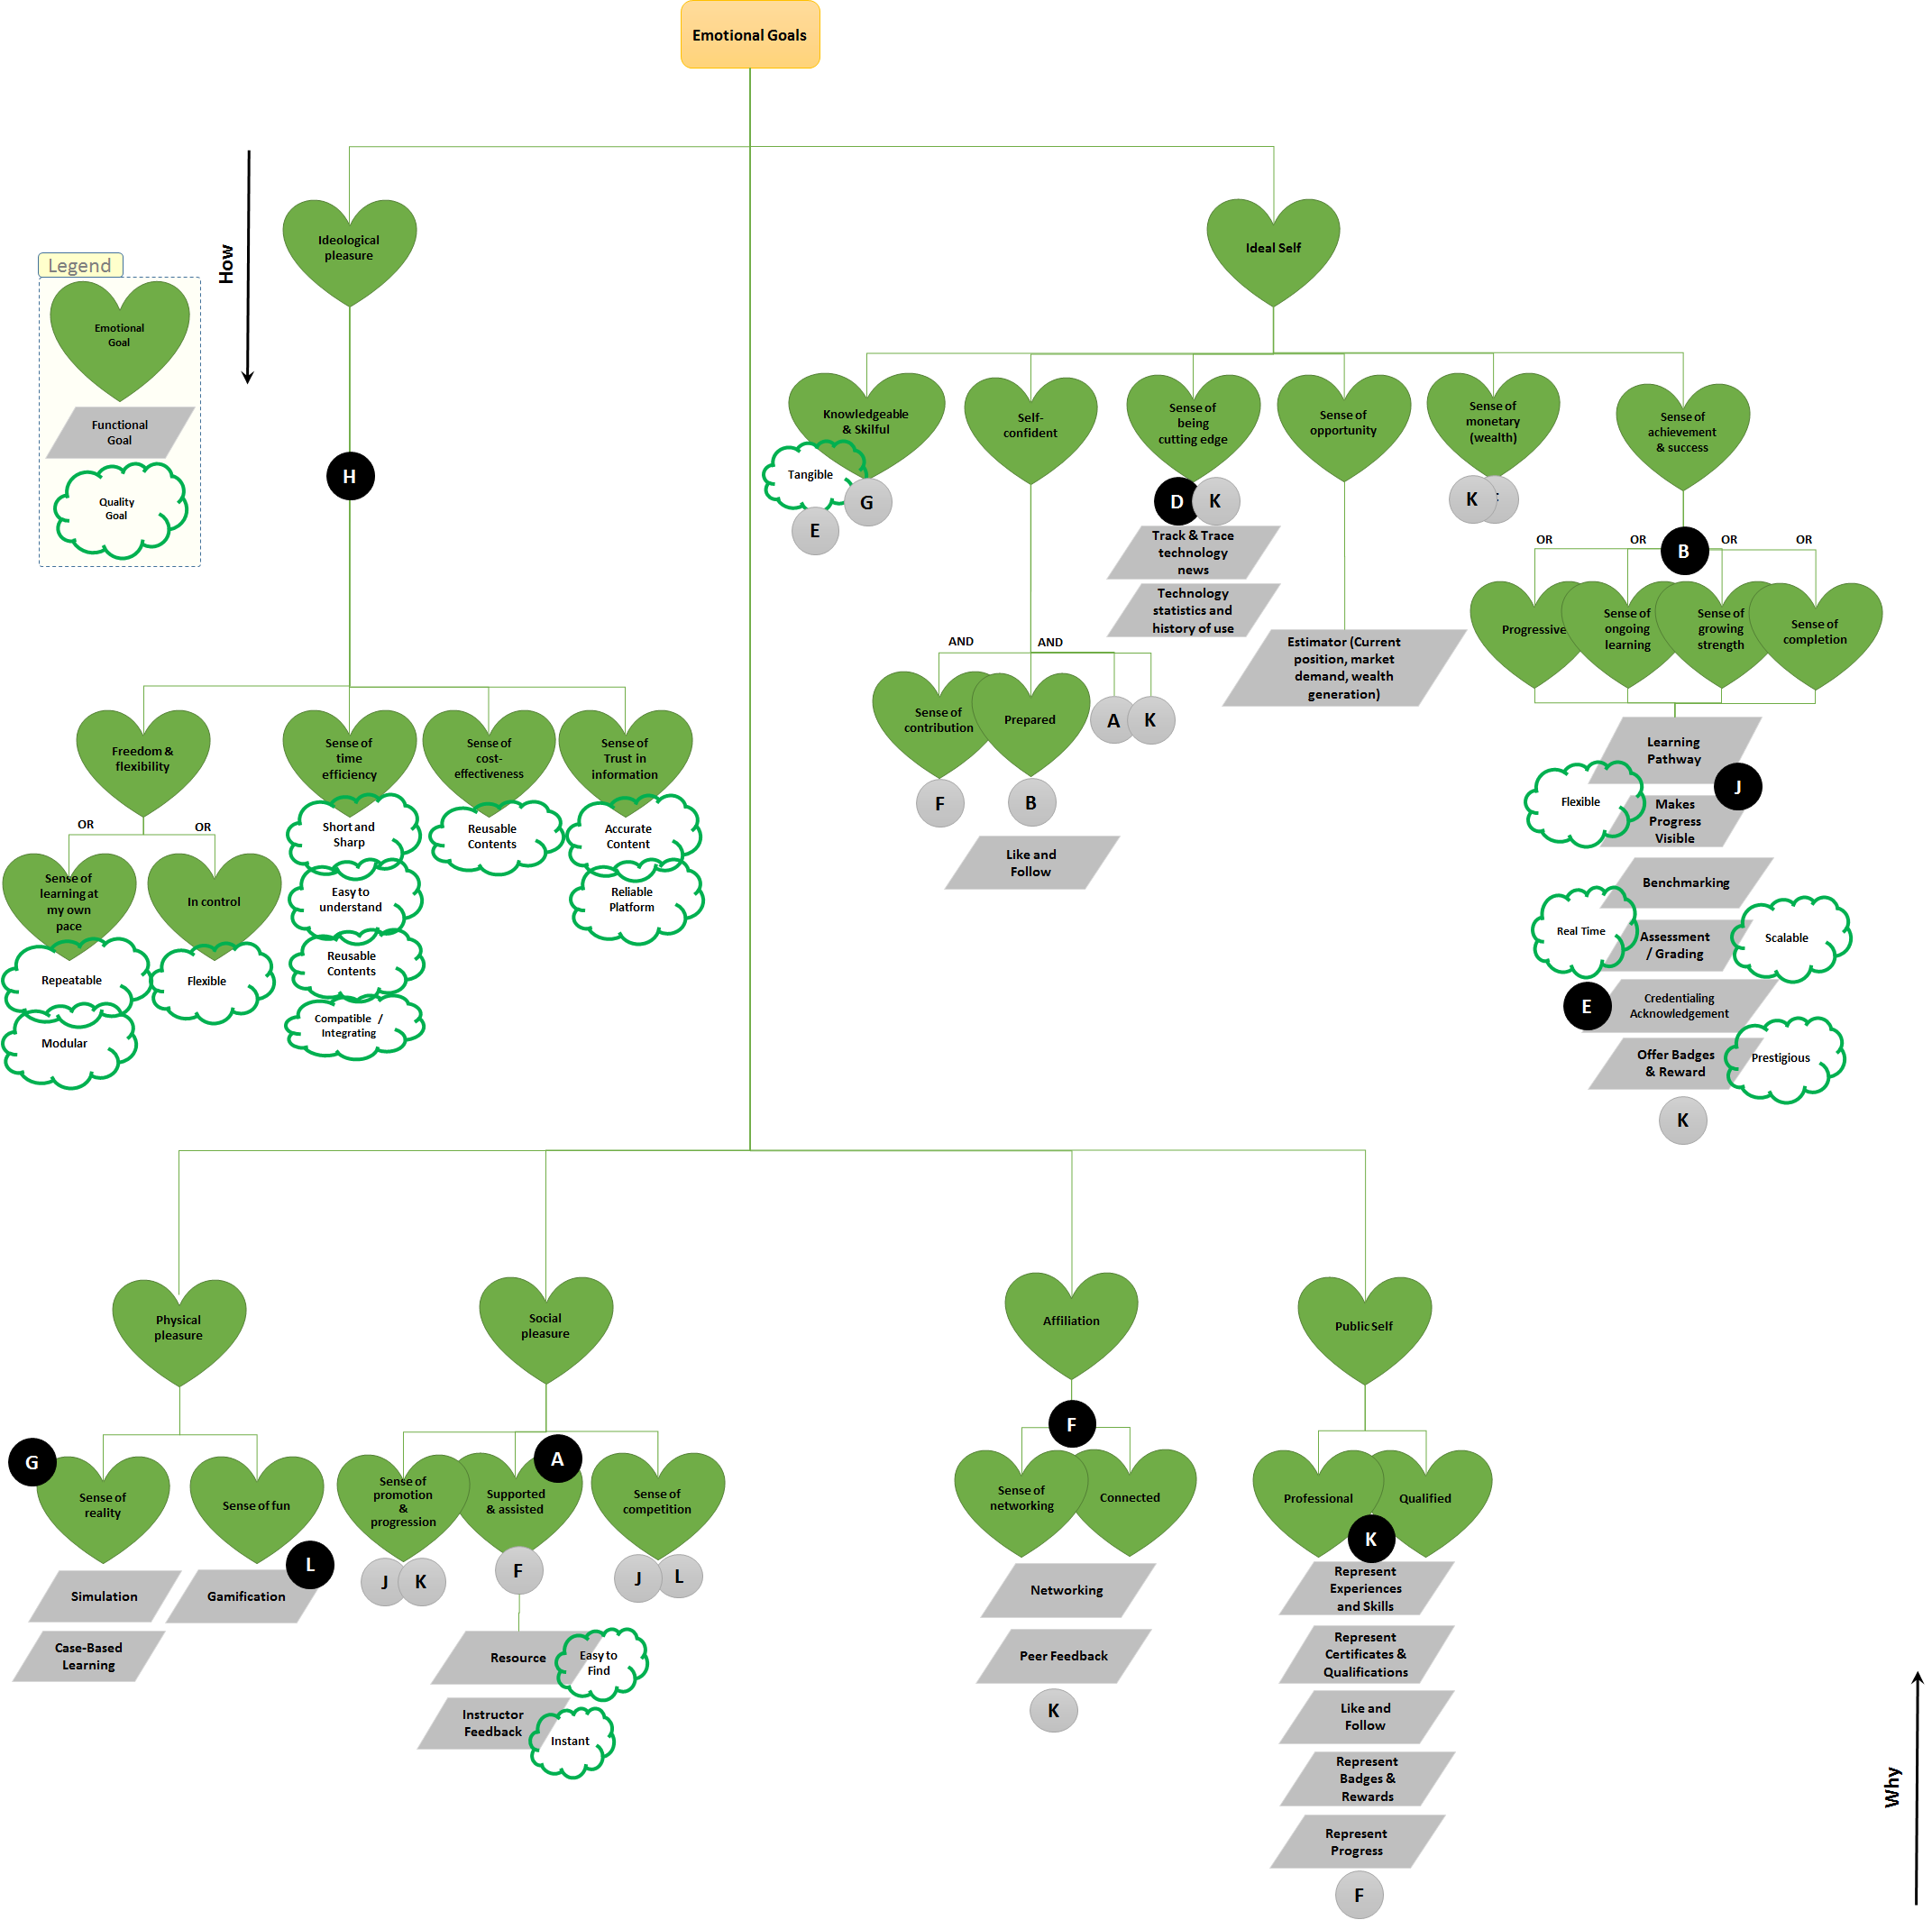}
\caption{\emph{Building Quality Passport} EG-SAT Analysis \\ (\emph{A high-resolution image is available at https://tinyurl.com/y842zja6})}
\label{fig:EG-SATAnalysis}
\end{figure*}
\end{landscape}
